# Supplementary material for: Diversity, Topology, and the Risk of Node Re-identification in Labeled Social Graphs
Source: arXiv:1808.10837 source file (2018-08-31)
Supplement: Supplementary file 1 [file appendix.tex]

\section*{Appendix}

\begin{figure*}[htb!]
	\centering
	\subfloat[Network: polblogs]{
		\includegraphics[scale=0.15]{pets18/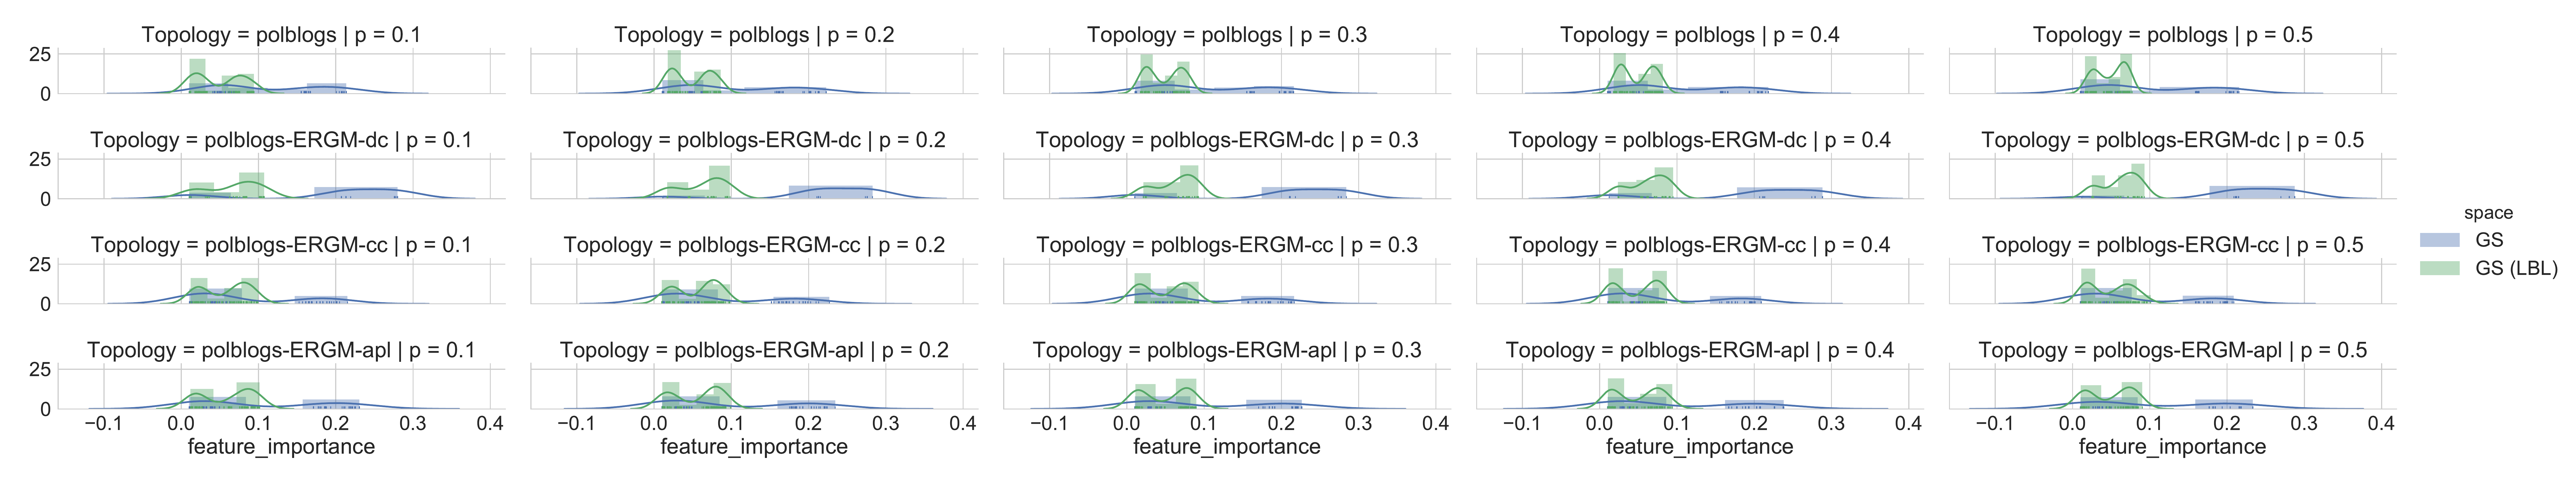}
			\label{fig:polblogs_syn_vulnerability_features}
	}
	\hspace{0mm}
\subfloat[Network: fb-caltech]{
	\includegraphics[scale=0.15]{pets18/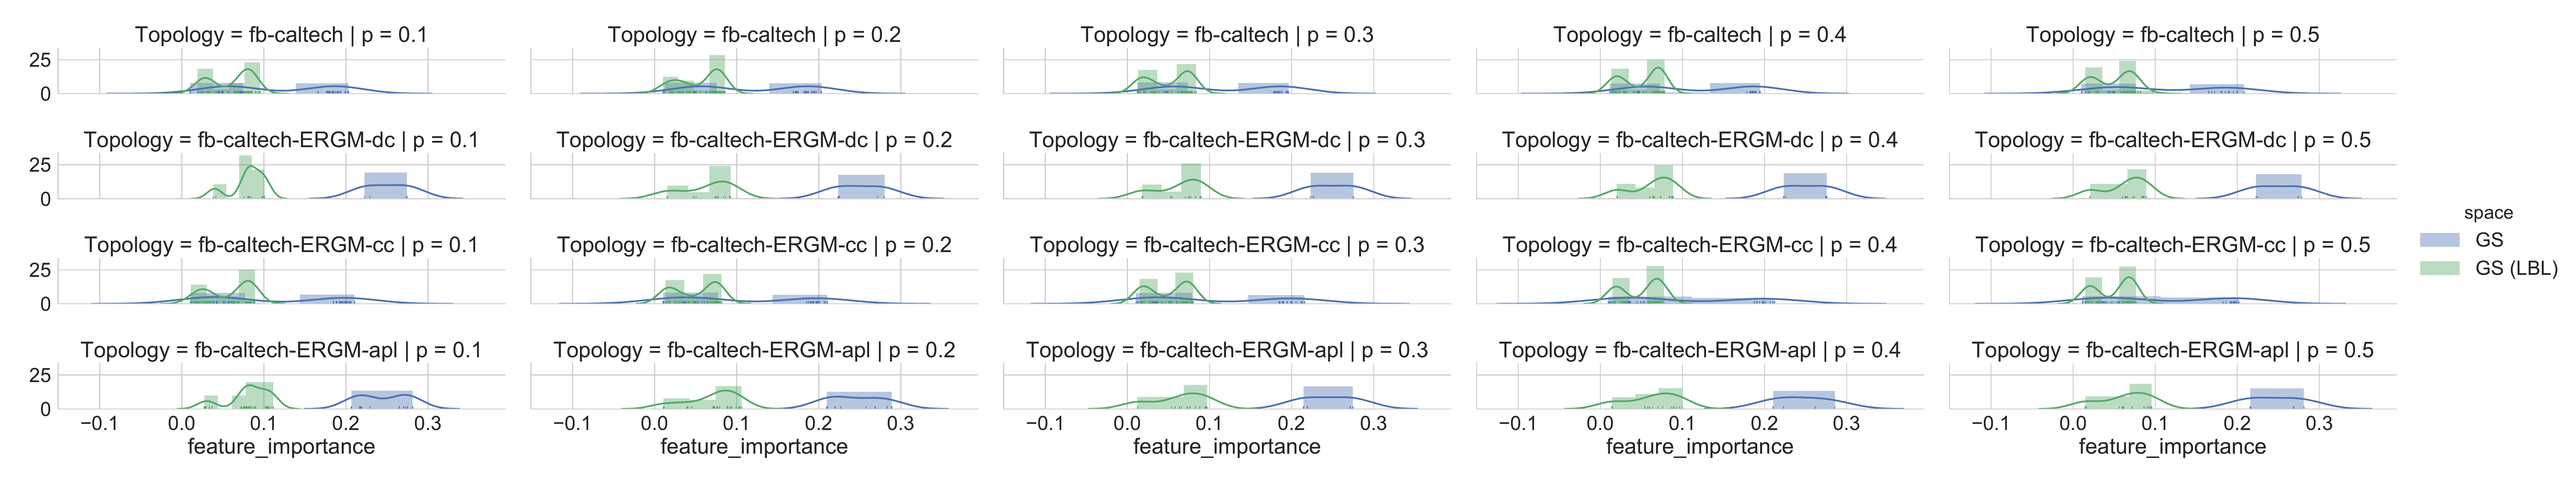}
			\label{fig:fb-caltech_syn_vulnerability_features}
}
\hspace{0mm}	
	
\subfloat[Network: fb-dartmouth]{
\includegraphics[scale=0.15]{pets18/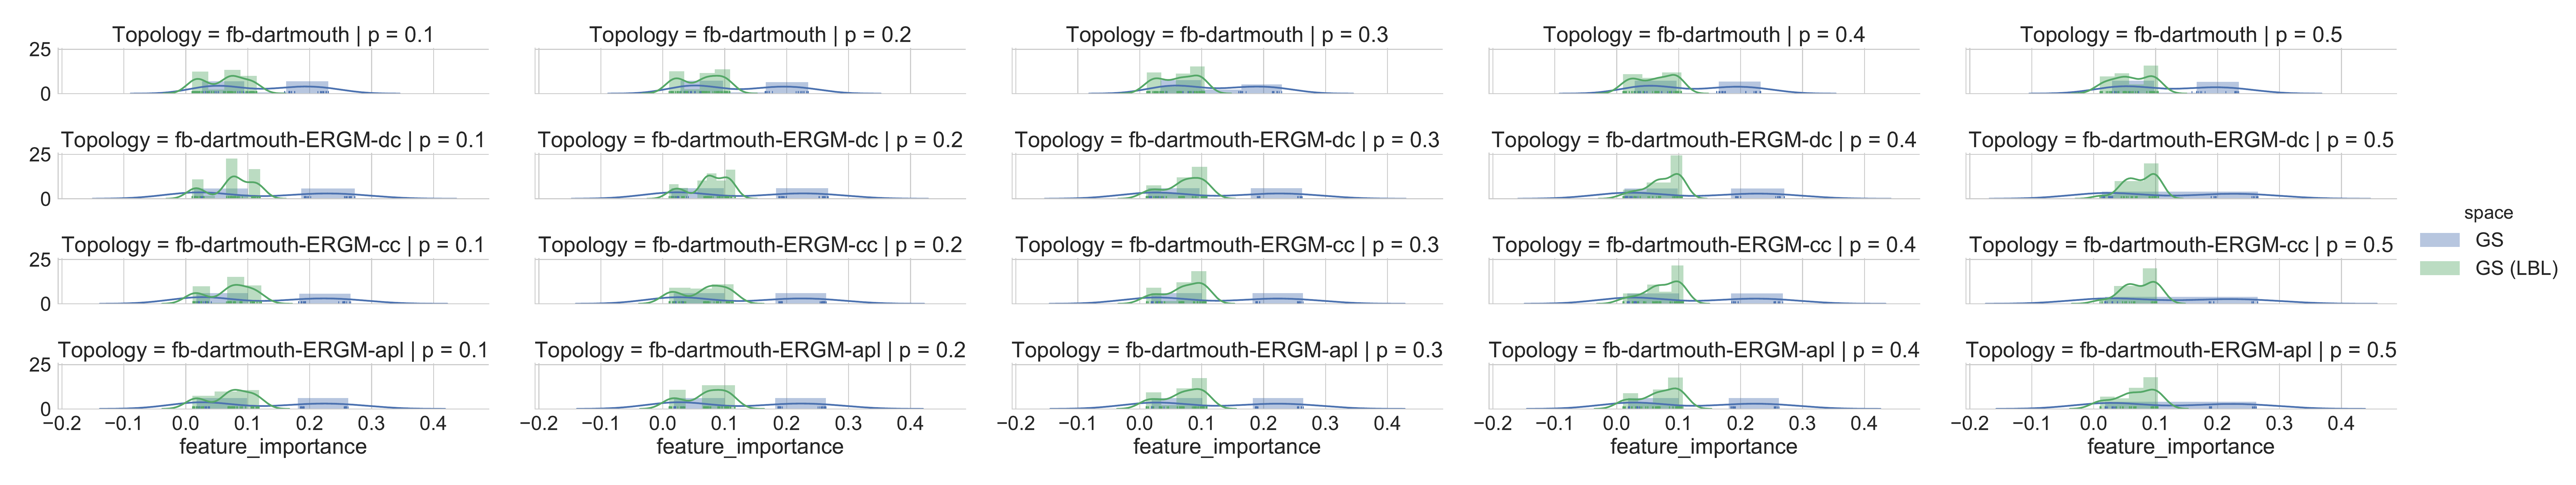}
			\label{fig:fb-dartmouth_syn_vulnerability_features}
}
\hspace{0mm}

\subfloat[Network: fb-michigan]{
\includegraphics[scale=0.15]{pets18/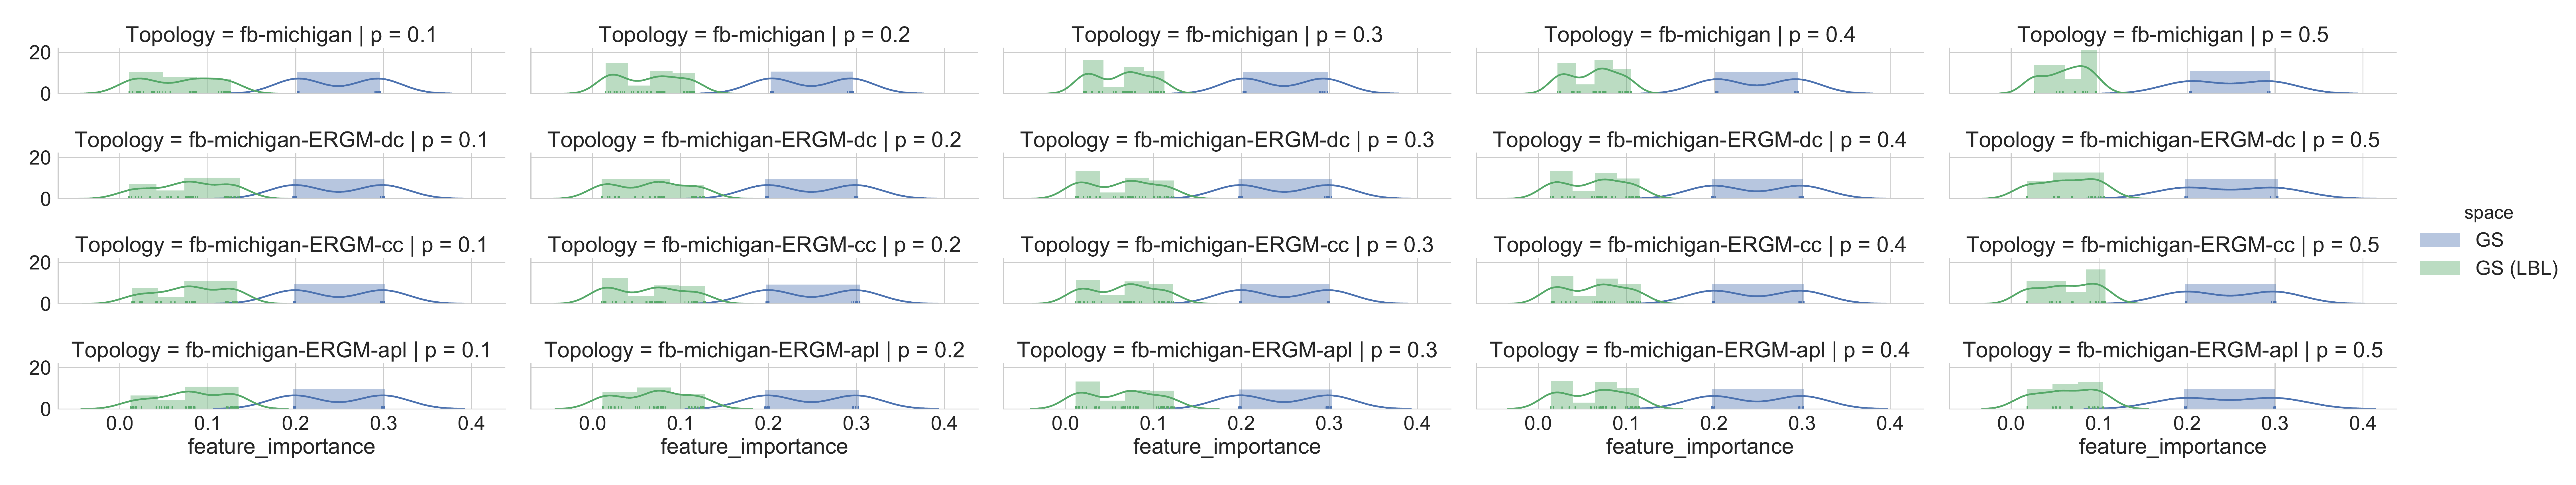}
			\label{fig:fb-michigan_syn_vulnerability_features}
}
\hspace{0mm}

\subfloat[Network: pokec-1]{
\includegraphics[scale=0.15]{pets18/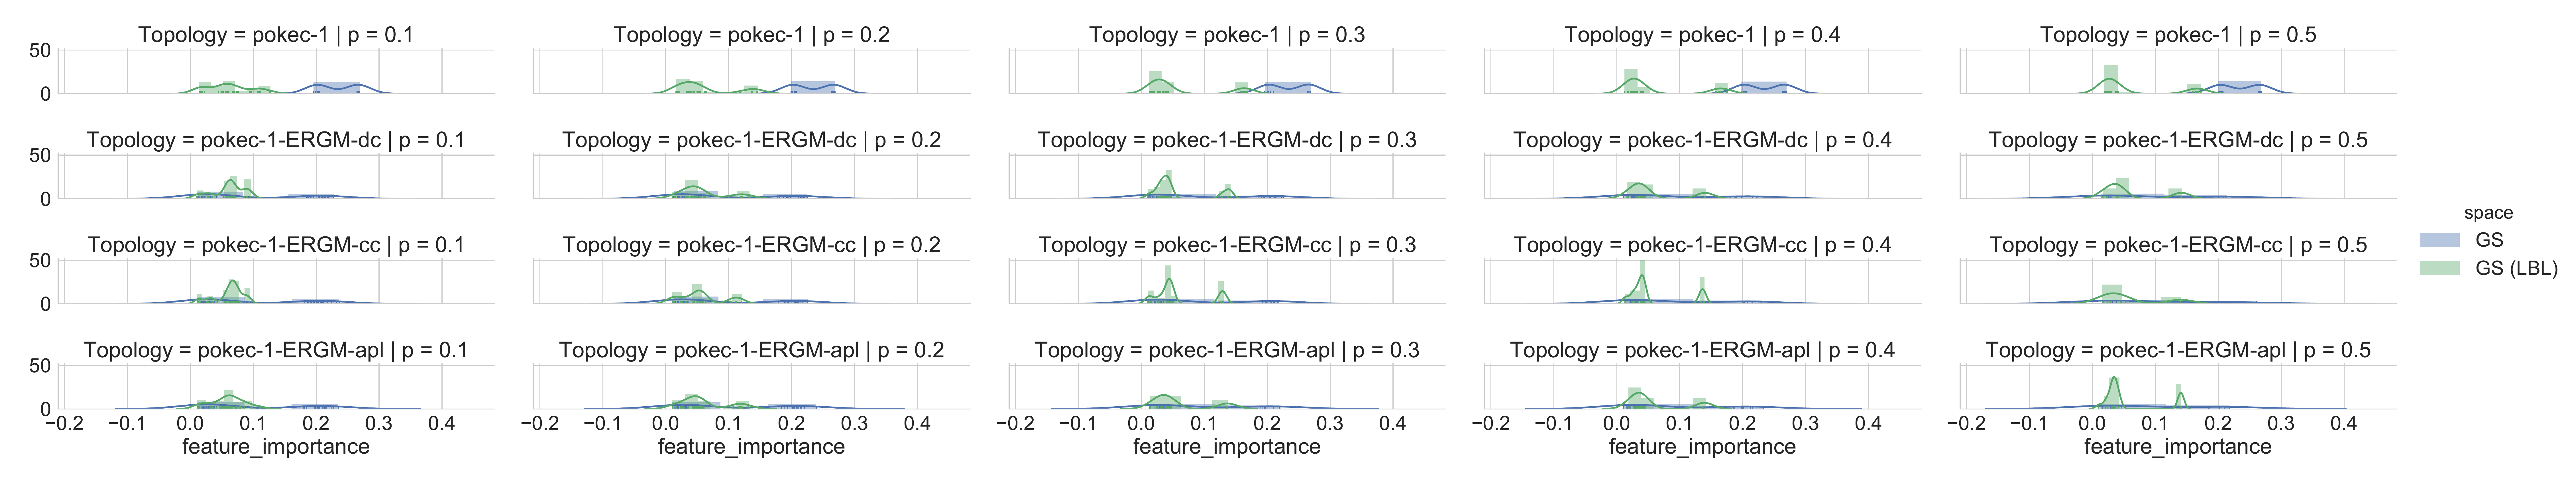}
			\label{fig:pokec-1_syn_vulnerability_features}
}
\hspace{0mm}

\subfloat[Network: amazon-products]{
\includegraphics[scale=0.15]{pets18/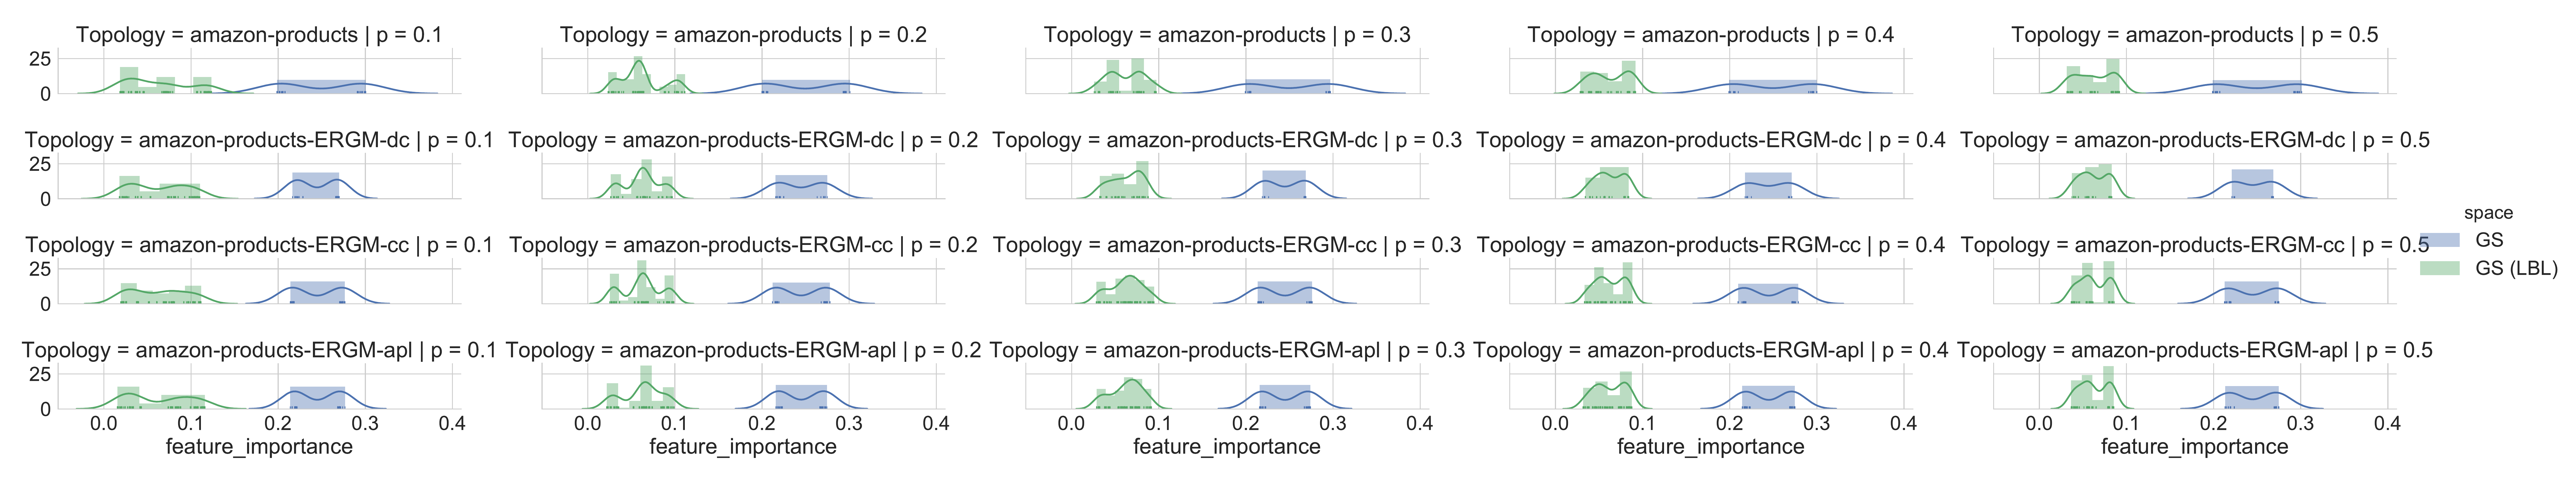}
			\label{fig:amazon-products_syn_vulnerability_features}
}
	 \caption{Kernel density estimate of the distribution of probability values which define the importance of features for the prediction tasks between original and ERGM graph structures. 
% 	 GS denotes the features based on the topology and GS (LBL) denotes the features based on both the topology and node attributes.
	}
	\label{fig:vulnerability_features_syn}
\end{figure*}

%\flush
